# Supplementary material for: Branch-Train-Merge: Embarrassingly Parallel Training of Expert Language Models
Source: arXiv:2208.03306 source file (2022-08-05)
Supplement: Supplementary file 1 [file averaging_results_scaling_appendix.tex]

% \begin{table*}[t]\small
% \centering
% % \resizebox{0.9\textwidth}{!}{
% \begin{tabular}{lcccc}
% \toprule
% &  \multicolumn{4}{c}{ \bf GPT-3 Small} \\
% \cmidrule{2-5}
% % % \emph{Shared Params}  & 124M & 124M & 96.1M & 67.8M  \\
% % % \emph{Expert Params}  & 0 & 0 & 28.3M & 56.7M  \\
% % % \emph{Total Params} & 124M & 124M & 322.8M & 521.1M  \\
% % \cmidrule{2-5}

% \textbf{Domain} & \bf \dataparallel  & \bf \domaintoken & \bf \plusmodelayers (L/2) & \bf \plusmodelayers (L) \\ %& \boldmath{\lnot}\textbf{\dapt}\\
% \midrule 

% \oneb 

% % 82.1
% & 14.6 & 14.2 & 14.3 & \bf 13.5  \\ %& 79.0$_{4.1}$\\

% \cs 
% % 82.1
% & 17.9 & 17.8 & 17.0 & \bf 15.6  \\ %& 79.0$_{4.1}$\\

% \legal 
% % 82.1
% & 10.5 & 10.1 &  9.5 & \bf 9.0   \\ %& 79.0$_{4.1}$\\

% \med  
% % 82.1
% & 13.8 & 14.1 & 13.4 & \bf 11.8 \\ %& 79.0$_{4.1}$\\

% \webtext 
% % 82.1
% & 22.0 & \bf 20.5 & 21.8 & 21.1 \\%& 79.0$_{4.1}$\\

% \realnews 
% % 82.1
% & 20.1 & \bf 18.6 & 20.0 &  18.8 \\ %& 79.0$_{4.1}$\\

% \reddit 
% % 82.1
% & 40.9 & \bf 40.3 & 41.6 &  40.8 \\ %& 79.0$_{4.1}$\\

% \reviews 
% % 82.1
% & 23.9 &  23.2 & 22.3 &  \bf 20.5\\ %& 79.0$_{4.1}$\\

% \midrule
% \bf Average & 20.5 & 19.9 &  20.0 & \bf 18.9 \\

% \bottomrule
% \end{tabular}
% % }
% \caption{Conditioning GPT-3 small on domains improves in-domain test performance, when training with 32 GPUs for 48 hours. See Appendix \label{sec:validation_curves} for validation curves during training.} 
% \label{tab:base_results}
% \end{table*}

\begin{table}[t]\small
\centering
% \resizebox{0.9\textwidth}{!}{
\begin{tabular}{rc}
\toprule
\multicolumn{2}{c}{\bf \# training domains }\\
&  64 \\
% &  \multicolumn{1}{p{0.5cm}}{\centering SM }  &  \multicolumn{1}{p{0.5cm}}{\centering MD \\ (64)} &  \multicolumn{1}{p{0.5cm}}{\centering LG \\ (128)} \\

\bf \denselm (350M)                  &  19.3\\
\bf \delm (350M; posterior weighted average)                  &  17.6 \\
\bf \delm (350M; posterior weights + greedy soup average)                  &   17.3 \\
\bf \denselm (1.3B)                    & 16.3 \\

\bottomrule \\
% \bf \dense XL (6144 GPU hours)      &   &   &    &   & \\
% \cmidrule{2-4}
% \bf \demixdapt (\S\ref{sec:dapt_improving_indomain}) & 17.7 & 14.6 & 13.7 \\
% \bf \densedapt (\S\ref{sec:dapt_improving_indomain}) & 69.0 & 21.0 & 17.4 \\

%& \boldmath{\lnot}\textbf{\dapt}\\

%&\boldmath{\lnot}\textbf{\dapt}\\
% \bf \plusdomainparallel (Mixed) & \bf 17.6 & \bf 14.7 & \bf 13.9 \\ %& \boldmath{\lnot}\textbf{\dapt}\\

% \bottomrule
\end{tabular}

% }
\caption{Comparing \delm{}s with expert averaging with the performance of \dense baselines on novel domains.Here we observe that expert averaging does not outperform output ensembling, but results in large gains in performance over dense models at a similar computational budget.}
\label{tab:averaging_results_scaling}
\end{table}
